# Supplementary material for: Growth of bilayer stanene on a magnetic topological insulator aided by a buffer layer
Source: arXiv:2310.08265 source file (2024-09-08)
Supplement: Supplementary file 1 [file SM_stanene_mbst_arxiv_R1.pdf]

# Supplementary material for manuscript entitled "Growth of bilayer stanene on a magnetic topological insulator aided by a buffer layer"

Sajal Barman[1,†], Pramod Bhakuni[1,†], Shuvam Sarkar[1], Joydipto Bhattacharya[2,3], Mohammad Balal[1], Mrinal Manna[1], Soumen Giri[1], Arnab Kumar Pariari[4], Tomáš Skála[5], Markus Hücker[4], Rajib Batabyal[1], Aparna Chakrabarti[2,3], and Sudipta Roy Barman[1*]

[1]*UGC-DAE Consortium for Scientific Research, Khandwa Road, Indore, 452001, India*

[2]*Theory and Simulations Laboratory, Raja Ramanna Centre for Advanced Technology, Indore 452013, Madhya Pradesh, India*

[3]*Homi Bhabha National Institute, Training School Complex, Anushakti Nagar, Mumbai 400094, Maharashtra, India*

[4]*Department of Condensed Matter Physics, Weizmann Institute of Science, Rehovot, Israel and*

[5]*Charles University, Faculty of Mathematics and Physics, V Holešovičkách 2, CZ-18000 Prague 8, Czech Republic.*

[†] Both authors contributed equally.

**The Supplementary Material consists of twenty nine figures Fig. S 1 to Fig. S 29, four tables Table S I to Table S IV.**

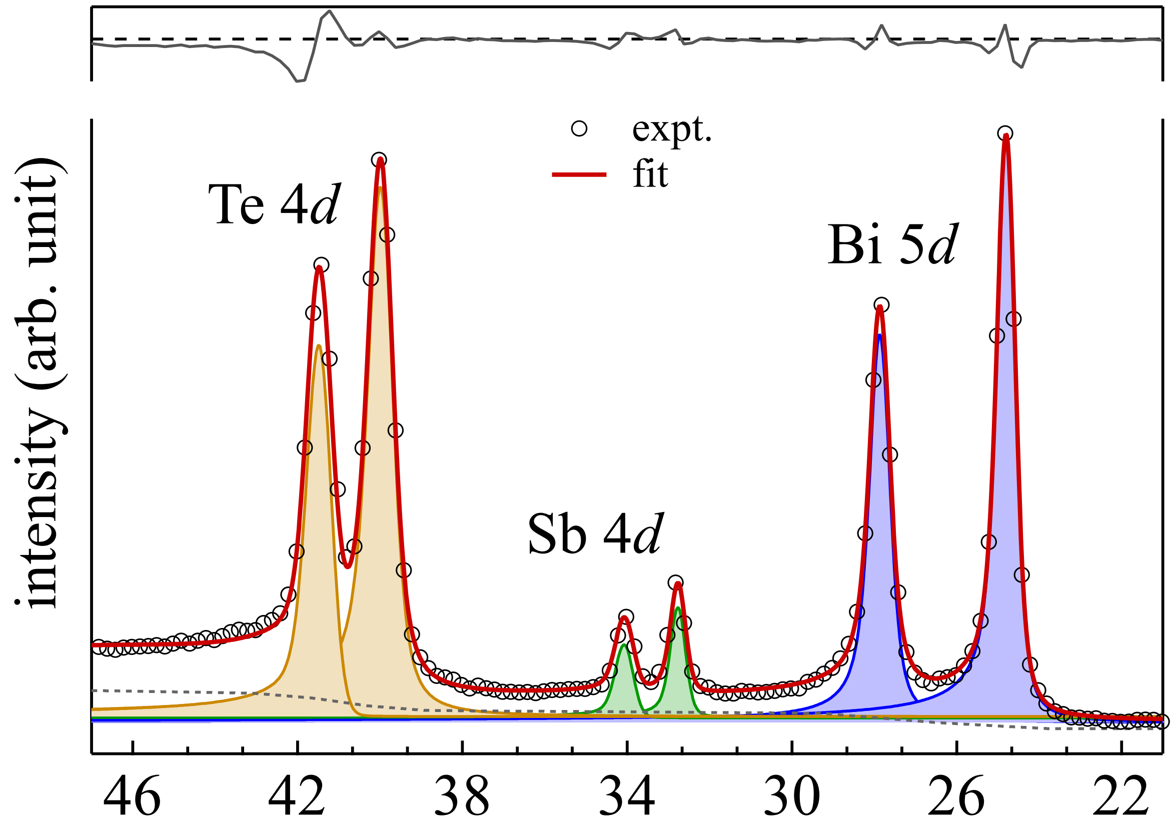


Fig. S 1. Bi 5*d*, Sb 4*d* and Te 4*d* HAXPES core level spectra (black open circles) of MBST measured with 6 keV photon energy. The fit (red curve) to the spectrum includes an inelastic background (black dashed curve). The residual of the fitting is shown in the top the panel. The Bi 5*d*, Sb 4*d*, and Te 4*d* core level peaks with spin-orbit splitting of 3.1, 1.3 and 1.5 eV are shown by blue, green and orange curves, respectively. A 30% Sb doping is obtained from the relative intensities of the peaks, as shown by the ratio of Bi:Sb:Te ≈ 0.7:0.3:2.

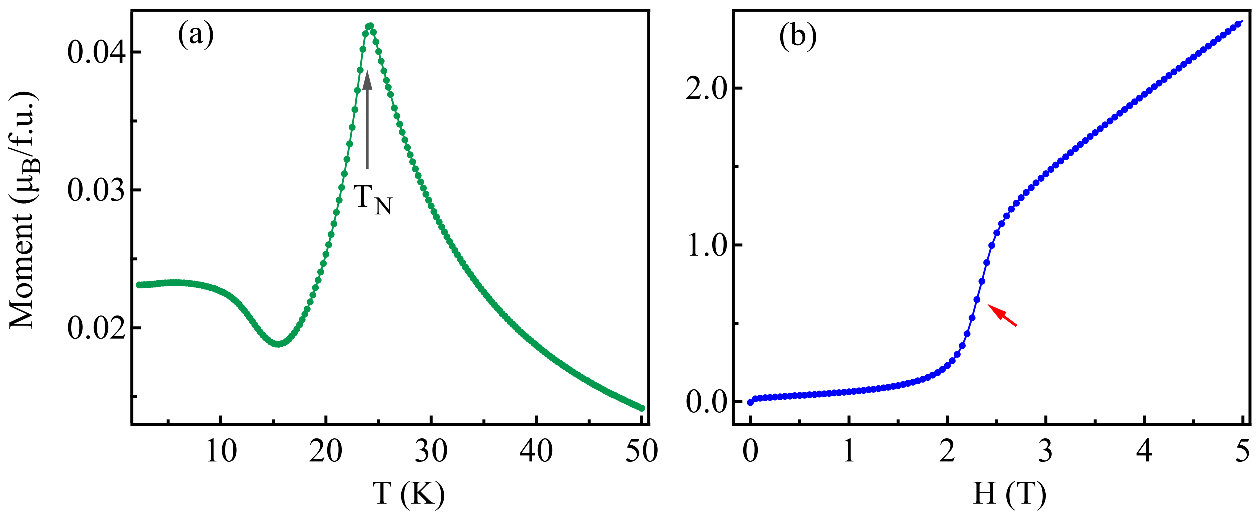


Fig. S 2. Magnetic characterization of MBST crystal with the magnetic field ($H$) parallel to the $c$-axis. (a) Magnetization ($M$) as a function of temperature at $H$= 0.1 Tesla, the gray arrow indicates the Neel temperature ($T_N$) to be 24 K. (b) $M(H)$ measurement at 2 K, the red arrow indicates the spin flop transition at 2.3 Tesla.

(a)

(b)

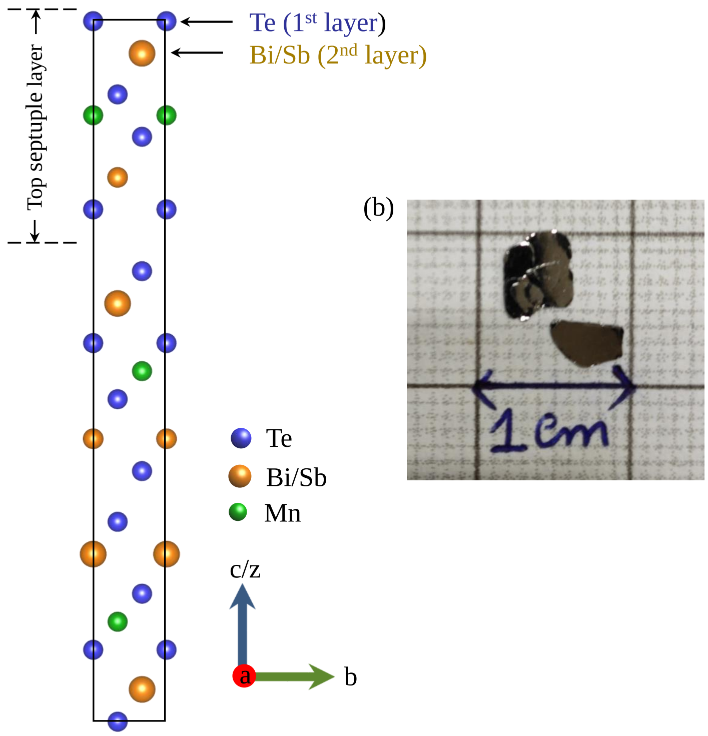


Fig. S 3. (a) The unit cell of $Mn(Bi_{0.7}Sb_{0.3})_2Te_4$ (MBST), where Te (Bi/Sb) constitutes top (second) layer of the (0001) surface. It has a $R\bar{3}m$ space group with lattice parameters $a$= 0.43 nm and $c$= 4.092 nm [1] consisting of three septuple layers that are coupled by van der Waals (vdW) interaction. (b) A photograph of the MBST crystals used in the present study.

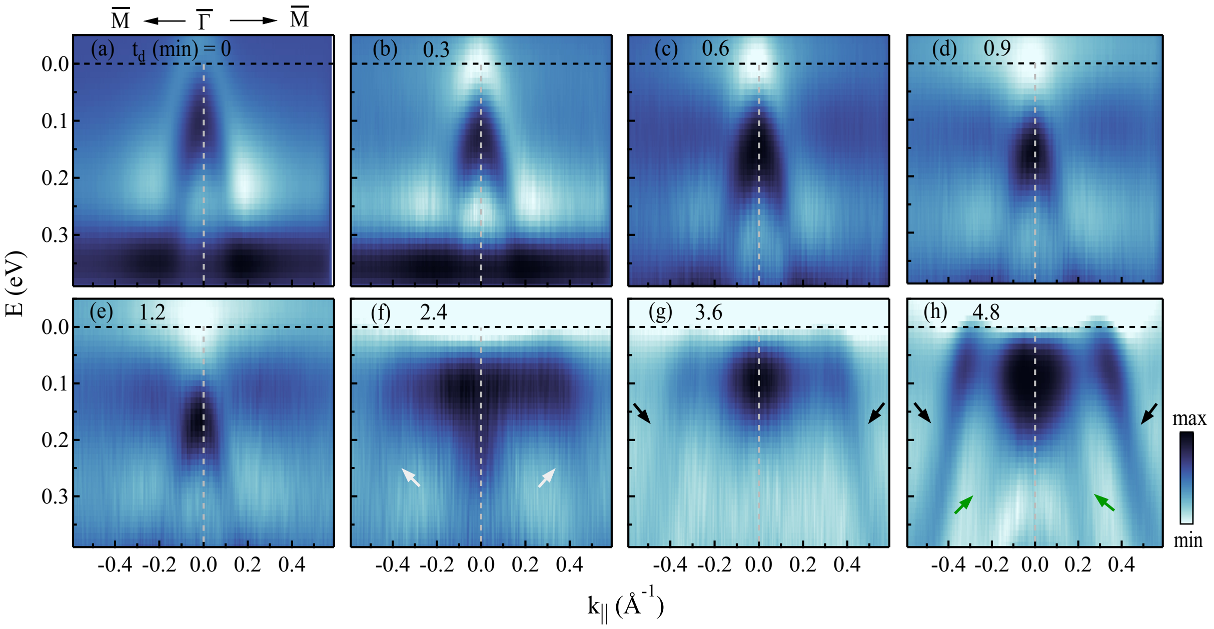


Fig. S 4. (a-h) The second derivative ARPES intensity plot towards $\overline{\Gamma}$-$\overline{M}$ direction corresponding to the raw data in Fig. 1 of the main manuscript. The black and green arrows highlight the outer and inner monolayer stanene bands, respectively. The white arrows in panel **f** indicate a BL related band. The color scale is shown on the right.

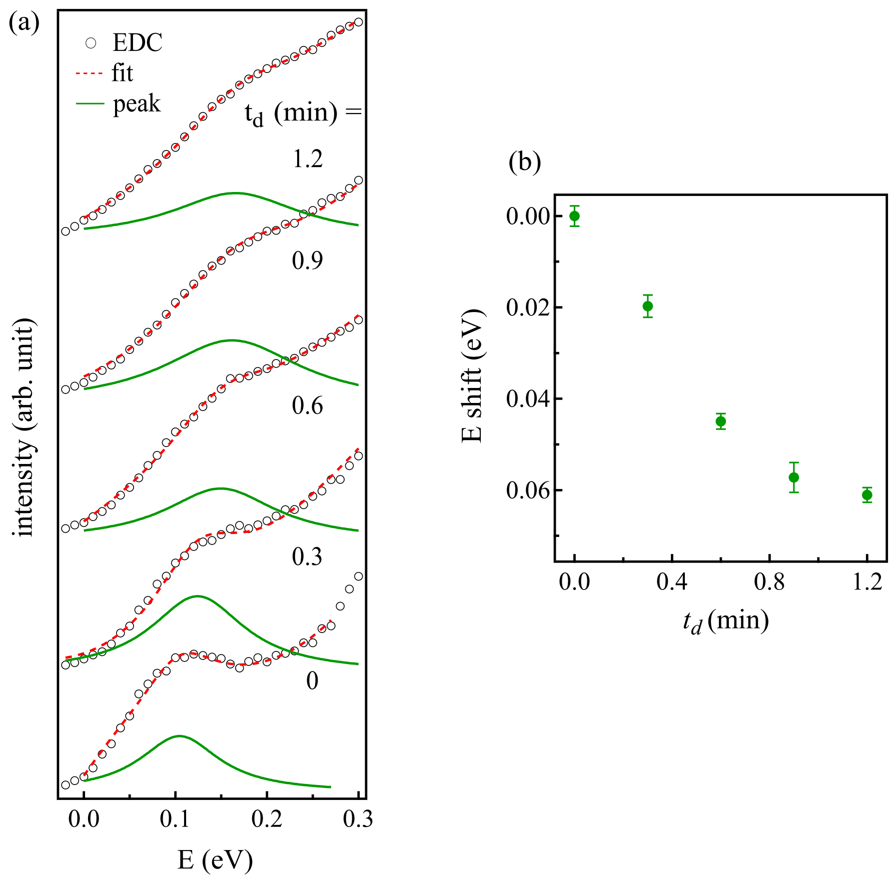


Fig. S 5. (a) The energy distribution curves (EDCs) of the raw ARPES spectra shown in Fig. 1 of the main text at $\overline{\Gamma}$ point, as a function of Sn deposition on MBST for different $t_d$. The maximum of the Lorentzian function (green curve) that has been used to fit the EDCs along with a linear background represents the band maximum. (b) The $E$ shift in the band maxima from panels **a** as a function of $t_d$.

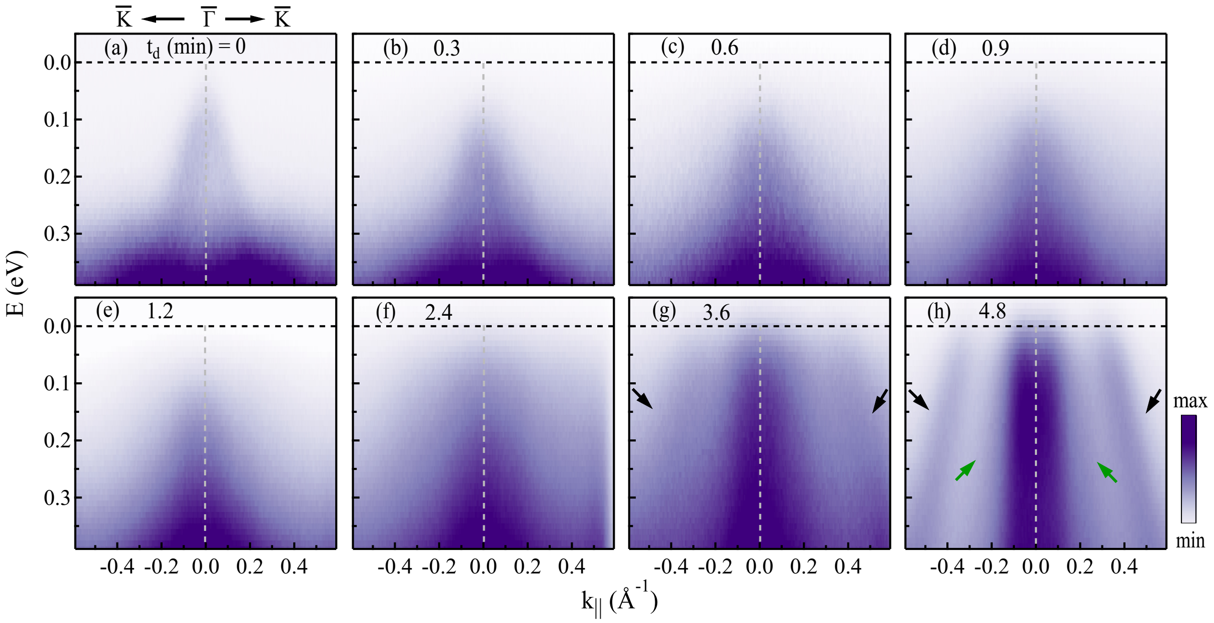


Fig. S 6. (a-h) The raw ARPES intensity plots towards $\overline{\Gamma}$-$\overline{K}$ for Sn deposition on MBST for different $t_d$. The black and green arrows highlight the outer and inner monolayer stanene bands, respectively. The color scale is shown on the right side.

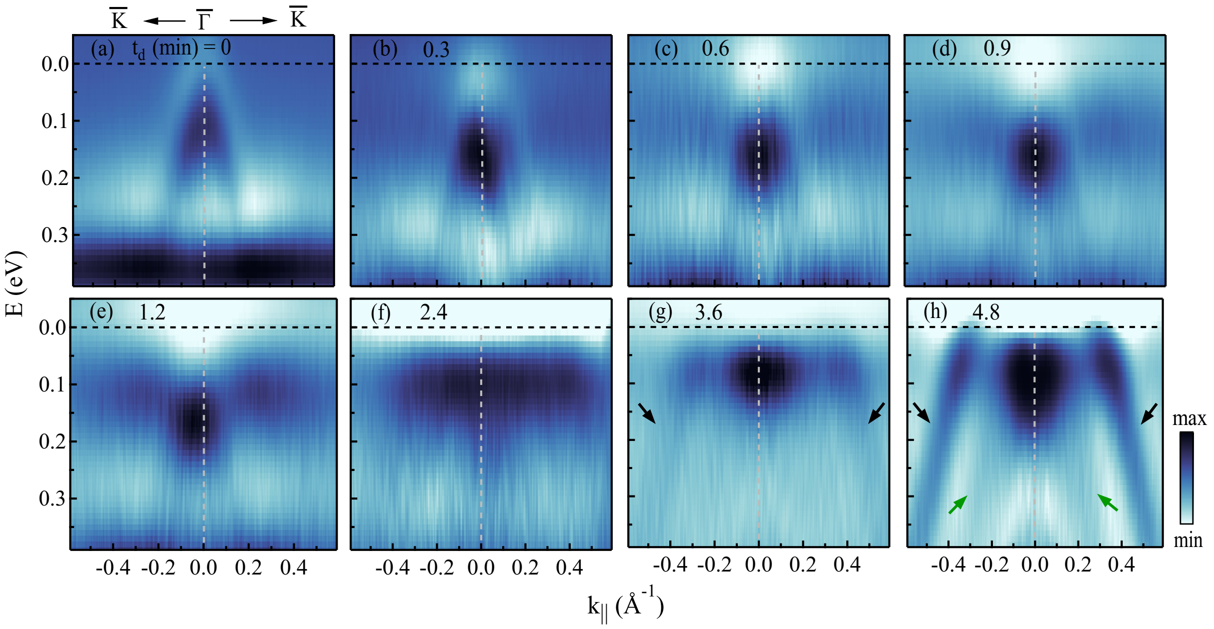


Fig. S 7. (a-h) The second derivative ARPES intensity plots towards $\overline{\Gamma}$-$\overline{K}$ for the raw data in Fig. S6 for Sn deposition on MBST for different $t_d$. The black and green arrows highlight the outer and inner monolayer stanene bands, respectively. The color scale is shown on the right side.

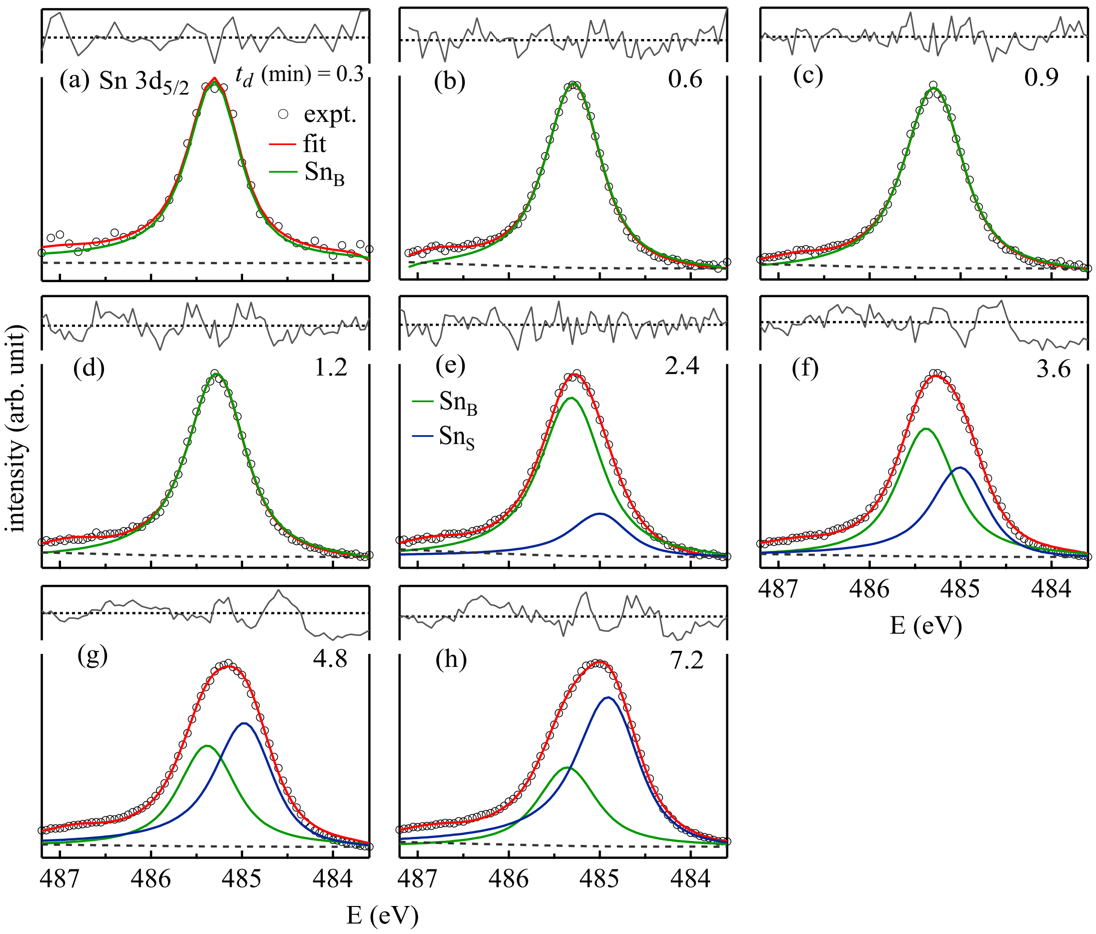


Fig. S 8. (a-h) Sn $3d_{5/2}$ XPS core level spectra at different Sn depositions are fitted by least square error minimization method. All the spectra are normalized to the same height. At the top of each panel, the residual of the fitting (gray curve) that exhibits random variation around zero (black dashed line) shows the good quality of the fit. An inelastic background that is included in the fitting is shown by black dashed curve.

Table S I. Parameters obtained from least square fitting of Sn $3d_{5/2}$ core level spectra, e.g., the binding energy ($E$), the life time broadening ($2\gamma$) of the components $Sn_B$, $Sn_S$ and the goodness of fit ($\chi^2$).

| $t_d$ (min) | E ± 0.025 (eV) | | $2\gamma$ ± 0.05 (eV) | | $\chi^2$ |
|---|---|---|---|---|---|
| components | $Sn_B$ | $Sn_S$ | $Sn_B$ | $Sn_S$ | |
| 0.3 | 485.29 | - | 0.49 | - | 0.033 |
| 0.6 | 485.27 | - | 0.55 | - | 0.009 |
| 0.9 | 485.28 | - | 0.60 | - | 0.012 |
| 1.2 | 485.27 | - | 0.60 | - | 0.011 |
| 2.4 | 485.30 | 484.97 | 0.65 | 0.56 | 0.006 |
| 3.6 | 485.38 | 484.97 | 0.60 | 0.55 | 0.013 |
| 4.8 | 485.38 | 484.94 | 0.60 | 0.60 | 0.014 |
| 7.2 | 485.36 | 484.87 | 0.60 | 0.67 | 0.007 |

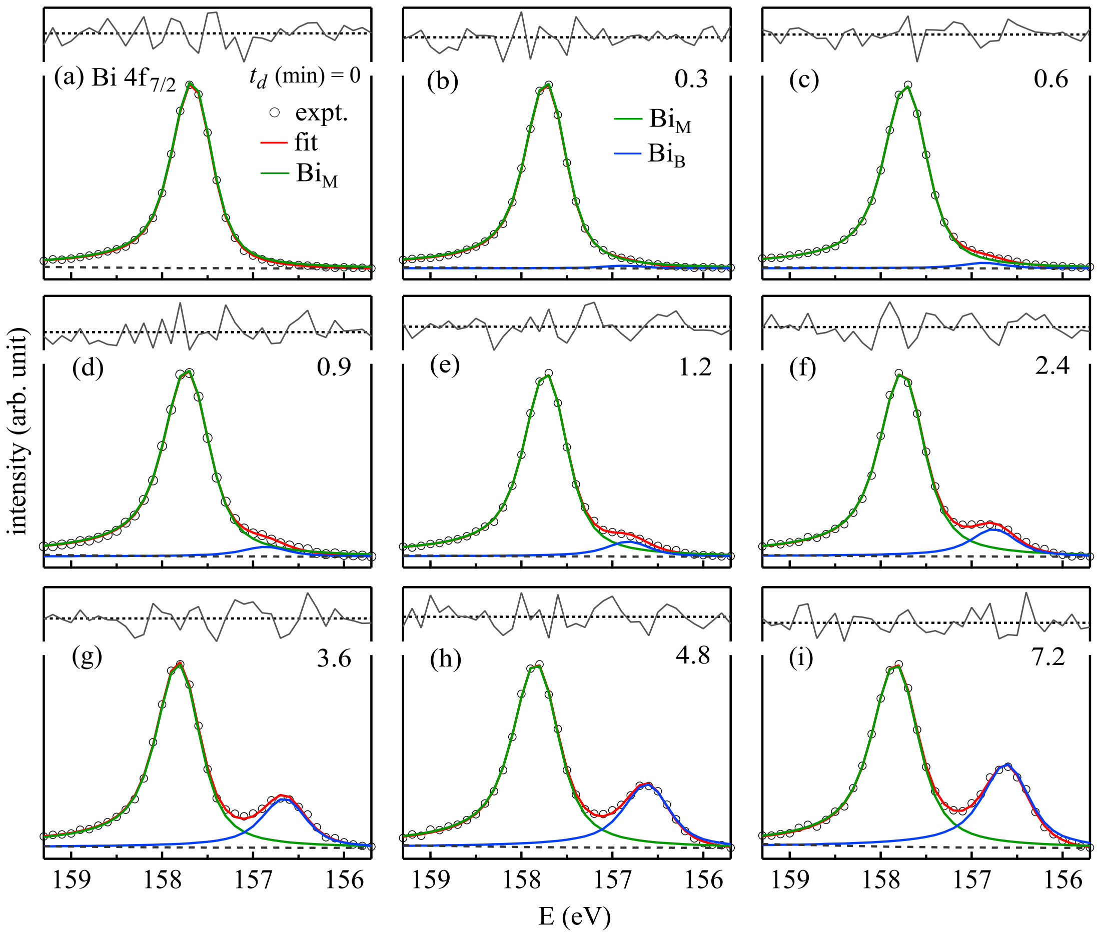


Fig. S 9. (a-i) Bi $4f_{7/2}$ XPS core level spectra at different Sn depositions are fitted by least square error minimization method. All the spectra are normalized to the same height. At the top of each panel, the residual of the fitting (gray curve) that exhibits random variation around zero (black dashed line) shows the good quality of the fit. An inelastic background that is included in the fitting is shown by black dashed curve.

Table S II. Parameters obtained from least square fitting of Bi $4f_{7/2}$ core level spectra, e.g., the binding energy ($E$), the life time broadening ($2\gamma$) of the components $Bi_M$, $Bi_B$ and the goodness of fit ($\chi^2$). $2\gamma$ was constrained to vary between 0.26 to 0.4 eV.

| $t_d$ (min) | E ± 0.025 (eV) | | $2\gamma$ ± 0.05 (eV) | | $\chi^2$ |
|---|---|---|---|---|---|
| components | $Bi_M$ | $Bi_B$ | $Bi_M$ | $Bi_B$ | |
| 0 | 157.65 | - | 0.28 | - | 0.005 |
| 0.3 | 157.71 | 156.85 | 0.29 | 0.29 | 0.005 |
| 0.6 | 157.71 | 156.85 | 0.32 | 0.32 | 0.008 |
| 0.9 | 157.71 | 156.85 | 0.37 | 0.37 | 0.003 |
| 1.2 | 157.72 | 156.80 | 0.33 | 0.33 | 0.003 |
| 2.4 | 157.75 | 156.74 | 0.36 | 0.36 | 0.004 |
| 3.6 | 157.80 | 156.64 | 0.34 | 0.34 | 0.005 |
| 4.8 | 157.82 | 156.60 | 0.38 | 0.38 | 0.004 |
| 7.2 | 157.82 | 156.60 | 0.39 | 0.39 | 0.003 |

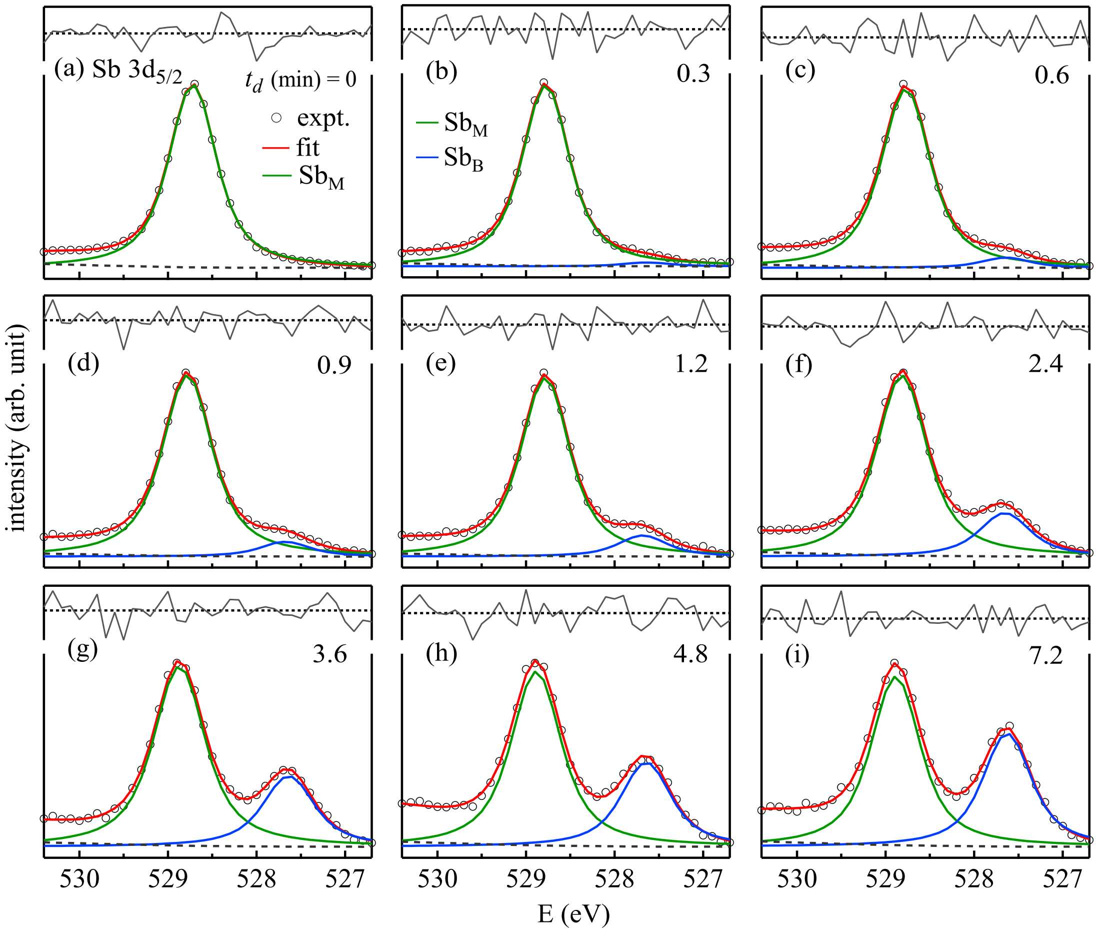


Fig. S 10. (a-i) Sb $3d_{5/2}$ XPS core level spectra at different Sn depositions are fitted by least square error minimization method. All the spectra are normalized to the same height. At the top of each panel, the residual of the fitting (gray curve) that exhibits random variation around zero (black dashed line) shows the good quality of the fit. An inelastic background that is included in the fitting is shown by black dashed curve.

Table S III. Parameters obtained from least square fitting of Sb $3d_{5/2}$ core level spectra, e.g., the binding energy ($E$), the life time broadening ($2\gamma$) of the components $Sb_M$, $Sb_B$ and the goodness of fit ($\chi^2$). $2\gamma$ was allowed to vary between 0.42 to 0.54 eV.

| $t_d$ (min) | E ± 0.025 (eV) | | $2\gamma$ ± 0.05 (eV) | | $\chi^2$ |
|---|---|---|---|---|---|
| components | $Sb_M$ | $Sb_B$ | $Sb_M$ | $Sb_B$ | |
| 0 | 528.72 | - | 0.46 | - | 0.002 |
| 0.3 | 528.77 | 527.64 | 0.46 | 0.46 | 0.004 |
| 0.6 | 528.77 | 527.64 | 0.48 | 0.48 | 0.002 |
| 0.9 | 528.78 | 527.68 | 0.50 | 0.50 | 0.004 |
| 1.2 | 528.79 | 527.68 | 0.48 | 0.48 | 0.004 |
| 2.4 | 528.81 | 527.66 | 0.52 | 0.52 | 0.006 |
| 3.6 | 528.87 | 527.64 | 0.53 | 0.53 | 0.007 |
| 4.8 | 528.88 | 527.64 | 0.51 | 0.51 | 0.013 |
| 7.2 | 528.89 | 527.63 | 0.50 | 0.50 | 0.014 |

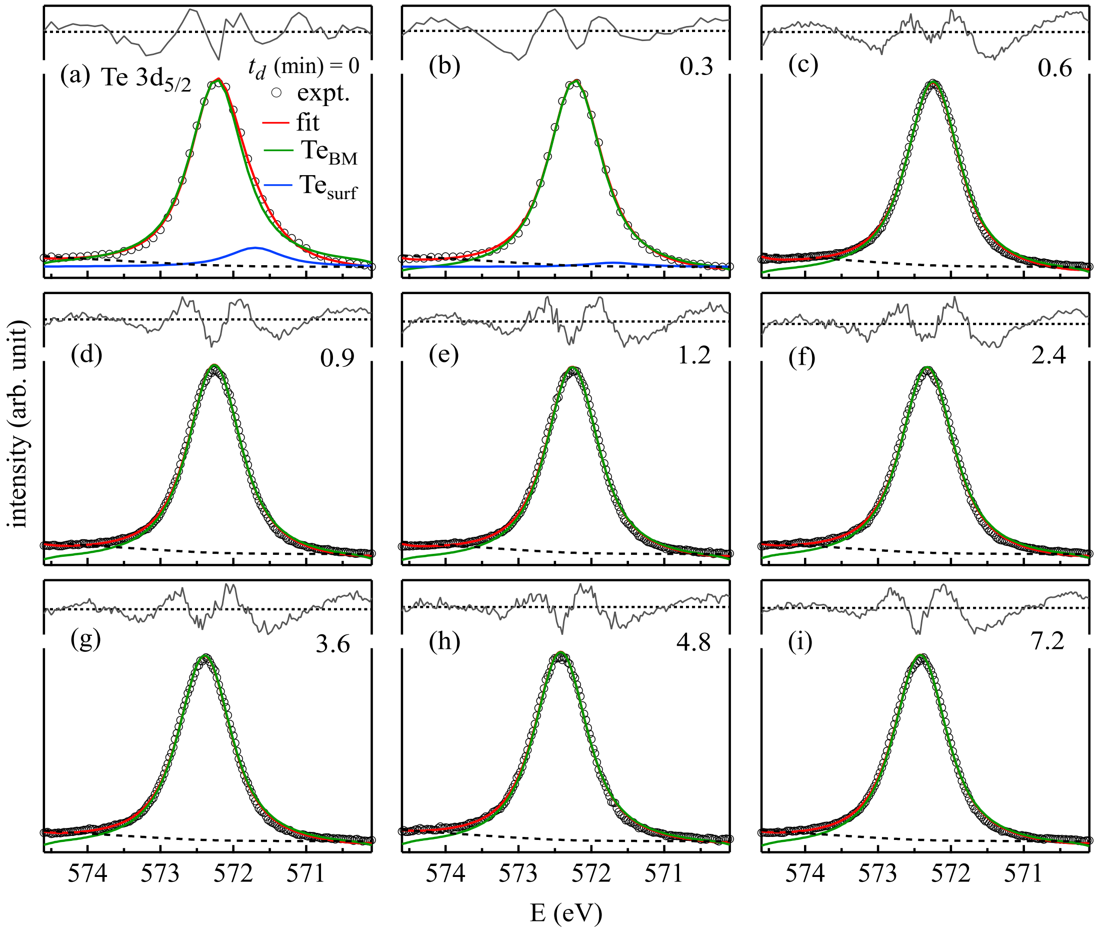


Fig. S 11. (a-i) Te $3d_{5/2}$ XPS core level spectra at different Sn depositions are fitted by least square error minimization method. All the spectra are normalized to the same height. At the top of each panel, the residual of the fitting (gray curve) that exhibits random variation around zero (black dashed line) shows the good quality of the fit. An inelastic background that is included in the fitting is shown by black dashed curve.

Table S IV. Parameters obtained from least square fitting of Te $3d_{5/2}$ core level spectra, e.g., the binding energy ($E$), the life time broadening ($2\gamma$) of the components $Te_{BM}$, $Te_{surf}$ and the goodness of fit ($\chi^2$).

| $t_d$ (min) | E ± 0.025 (eV) | | $2\gamma$ ± 0.05 (eV) | | $\chi^2$ |
|---|---|---|---|---|---|
| components | $Te_{BM}$ | $Te_{surf}$ | $Te_{BM}$ | $Te_{surf}$ | |
| 0 | 572.23 | 571.70 | 0.75 | 0.75 | 0.005 |
| 0.3 | 572.23 | 571.70 | 0.75 | 0.75 | 0.004 |
| 0.6 | 572.25 | - | 0.72 | - | 0.026 |
| 0.9 | 572.26 | - | 0.76 | - | 0.032 |
| 1.2 | 572.26 | - | 0.74 | - | 0.029 |
| 2.4 | 572.32 | - | 0.75 | - | 0.032 |
| 3.6 | 572.39 | - | 0.75 | - | 0.029 |
| 4.8 | 572.42 | - | 0.75 | - | 0.035 |
| 7.2 | 572.42 | - | 0.75 | - | 0.035 |

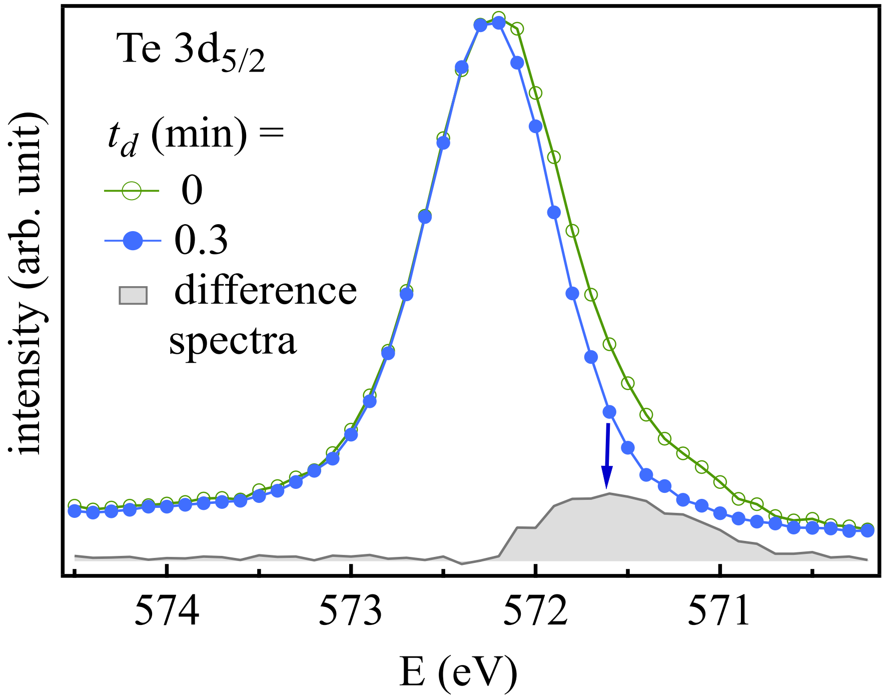


Fig. S 12. Te 3$d_{5/2}$ core level spectra of MBST ($t_d$= 0) compared to that for Sn deposition of 0.3 min, both normalized to the same height. Their difference spectrum (gray shaded) represents the surface core level peak, the peak position is shown by a blue arrow.

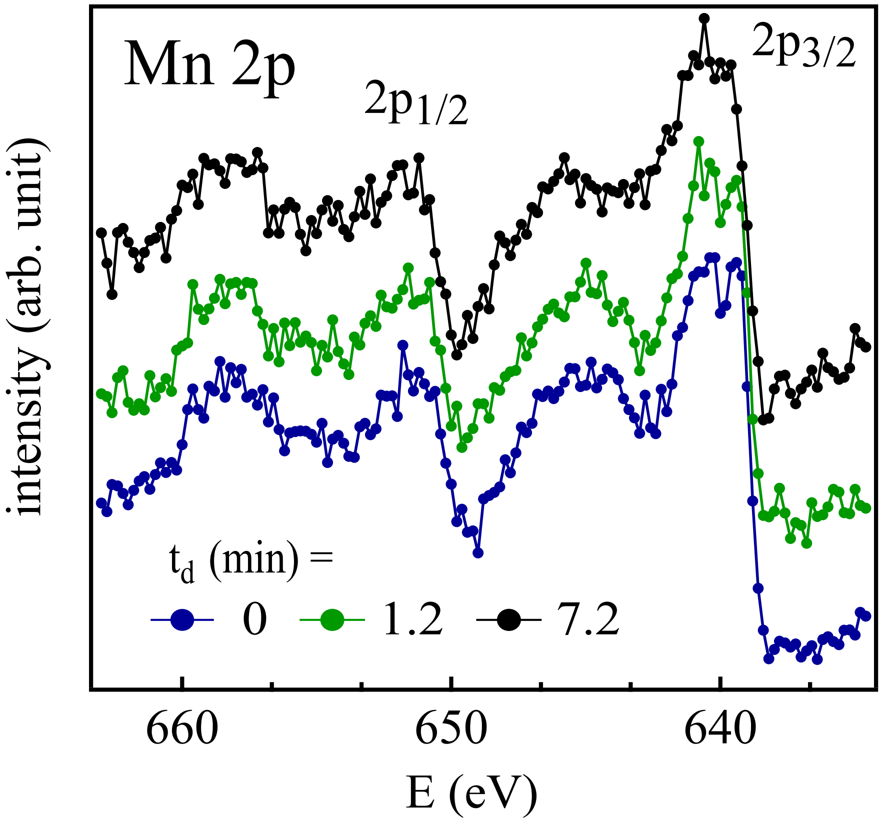


Fig. S 13. Mn 2*p* XPS core level spectra for different $t_d$ compared to that of MBST. All the spectra are normalized to the same height.

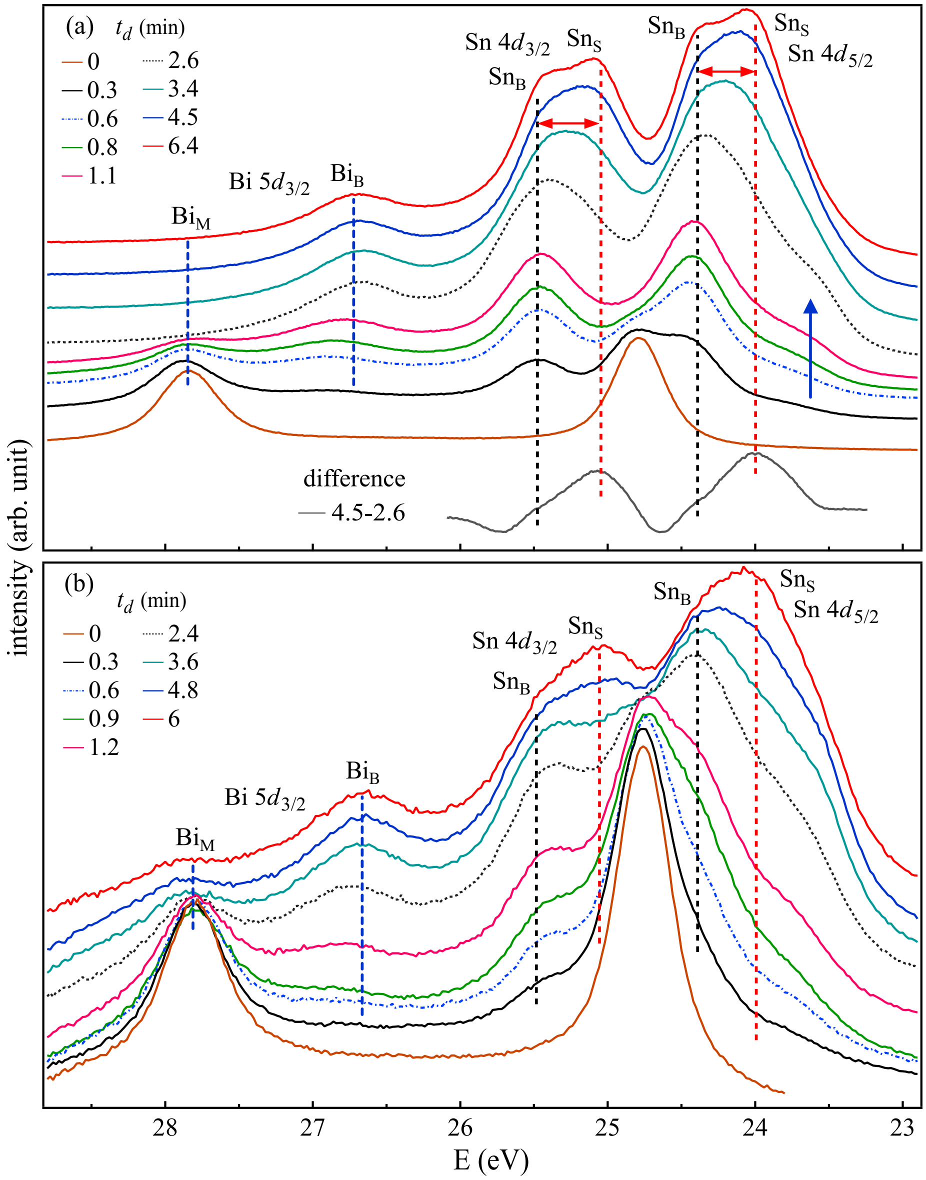


Fig. S 14. Sn 4$d$ and Bi 5$d$ shallow core level spectra taken with (a) 90 eV (synchrotron radiation) and (b) 40.8 eV (He II radiation) photon energies. $t_d$ of the former is scaled with the latter. The stanene related $Sn_S$ components (BL related $Sn_B$) for both the spin orbit components of Sn 4$d$ are shown by red (black) dashed lines and also by the difference spectrum between primarily monolayer stanene ($t_d$= 4.5 min) and BL ($t_d$=2.6 min). The $Bi_B$ and $Bi_M$ components of Bi $5d_{3/2}$ are shown by blue dashed lines ($Bi_B$ component of Bi $5d_{5/2}$ is shown by blue arrow).

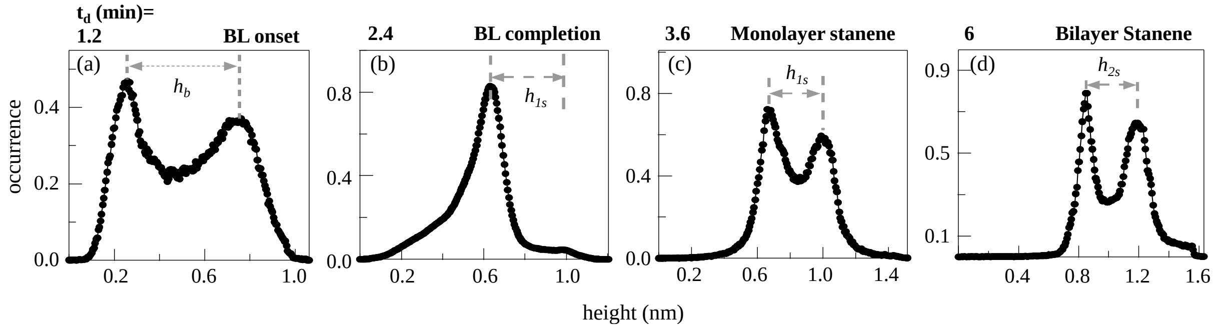


Fig. S 15. The height histograms corresponding to Figs. 3(a-d), respectively of the main manuscript. $h_b$, $h_{1s}$, $h_{2s}$ represent the heights of the buffer layer, monolayer stanene and the bilayer stanene, respectively.

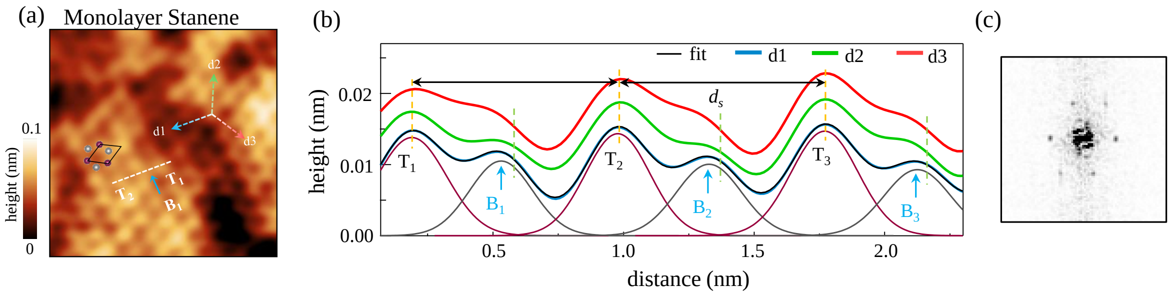


Fig. S 16. (a) An atomically resolved image of monolayer stanene region for $t_d$= 3.6 min (4 nm × 4 nm, $I_T$= 0.8 nA, $U_T$= -0.75 V). (b) Average height profiles for panel **a** along d1, d2 and d3 directions, the former is fitted with Gaussian functions, symbols have same meaning as Fig. 3(j) of main manuscript. (c) The Fourier transform of panel **a**.

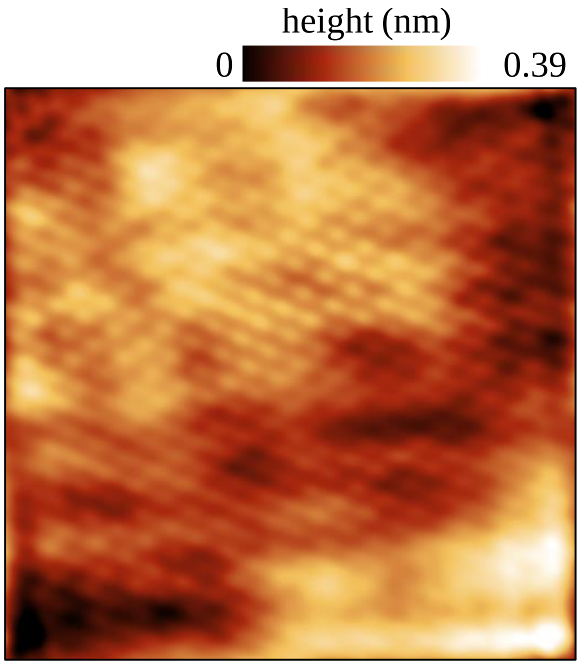


Fig. S 17. Atomic resolution STM topography of the BL for $t_d$= 2.4 min (10 nm × 10 nm with $I_T$ = 0.49 nA and $U_T$ = -0.15 V). The dark region in the lower left corner is the uncovered substrate.

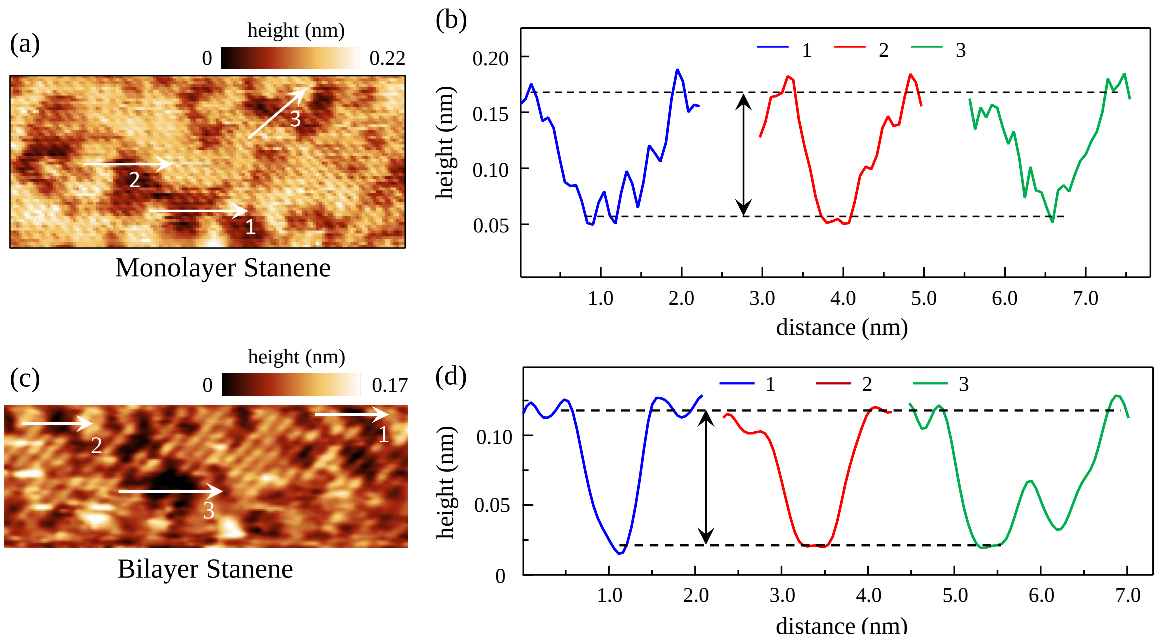


Fig. S 18. (a) STM topography (9 nm × 4.3 nm, $I_T$= 0.57 nA, and $U_T$= 0.06 V) for monolayer stanene. (b) Height profiles across the upper and lower sublattice along the white arrows numbered 1-3 in panel **a**. (c) STM topography (11 nm × 3.8 nm, $I_T$= 0.45 nA, and $U_T$= -0.7 V) for bilayer stanene. (d) Height profiles across the upper and lower sublattice along the white arrows numbered 1-3, as shown in panel **c**. The buckling height turns out to be 0.1±0.015 nm.

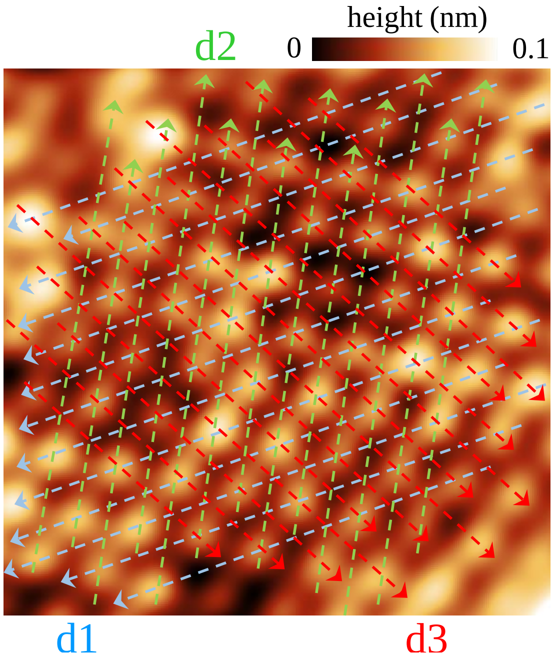


Fig. S 19. The atomic resolution STM image of bilayer stanene (4 nm × 4 nm, same as Fig. 3(i) of main manuscript) shown overlaid by dashed blue, green and red lines along the d1, d2, and d3 directions, respectively along which the height profiles have been taken for averaging.

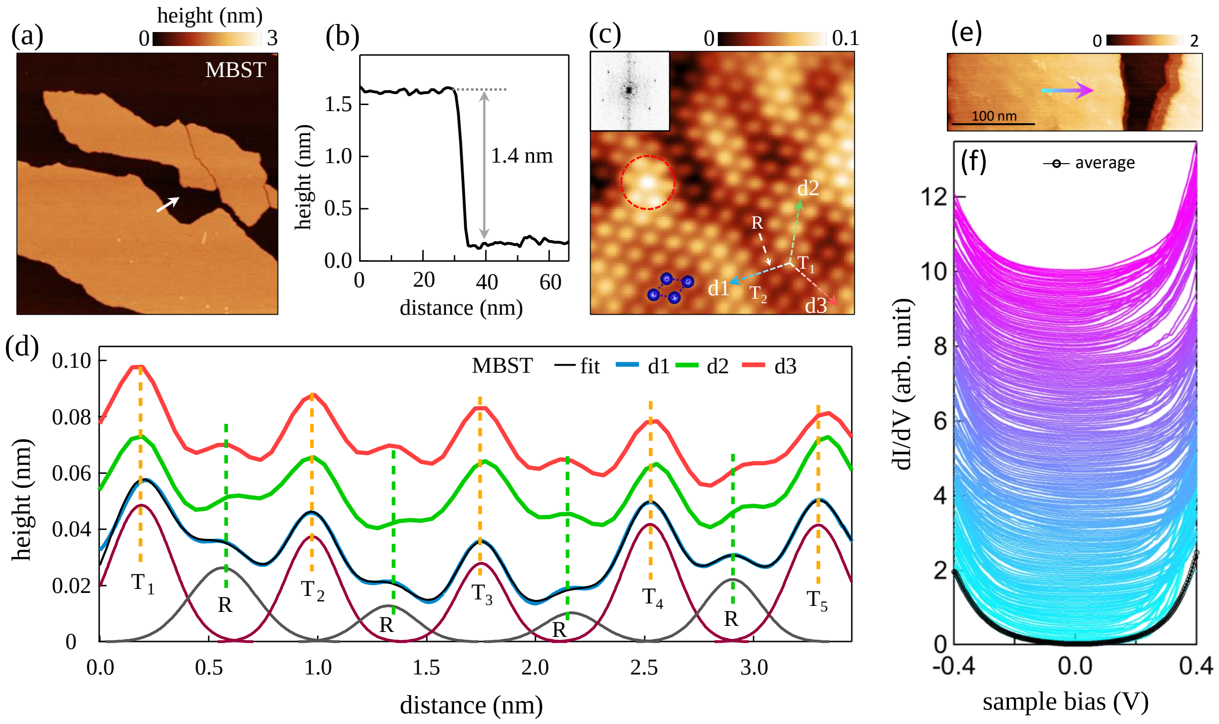


Fig. S 20. (a) Wide area STM topography (400 nm × 400 nm with tunneling current $I_T$= 0.2 nA and $U_T$= -0.8 V) of the Te terminated MBST surface. (b) A height profile extracted along the white arrow shown in panel **a** quantifies the step height to be 1.4±0.03 nm, which is close to the 1.36 nm height of a single septuple layer of MBST shown in Fig. S3. (c) Atomic resolution STM image of the MBST surface (5 nm × 5 nm with $I_T$= 0.7 nA and $U_T$= 0.4 V) , inset shows the Fourier transform of this image. The unit cell is shown by blue dashed lines, blue circles represent Te atoms. A bright protrusion highlighted by a red dashed circle indicates presence of $(Bi/Sb)_{Te}$ anti-site defect. (d) Height profiles from the atomic resolution image along the three different directions (d1, d2, d3), as shown in panel **c**. The profiles are fitted with Gaussian functions of nearly similar FWHM, fitting along d1 is shown by a black curve, where the peaks $T_n$, n= 1-4 (magenta curves) represent the atom positions and peaks indicated by R (gray curves) are attributed to the residual contribution that appears in the middle of $T_nT_{n+1}$. (e) STM topography image (300 nm × 90 nm, $I_T$ = 0.1 nA and $U_T$ = -0.4 V) of the MBST surface with an horizontal arrow of length of 73 nm along which $dI/dV$ scanning tunneling spectra (STS) were taken at 201 equally separated points. (f) The waterfall plot of the STS spectra taken along the arrow in panel **e**, the black curve represents the average of all the spectra.

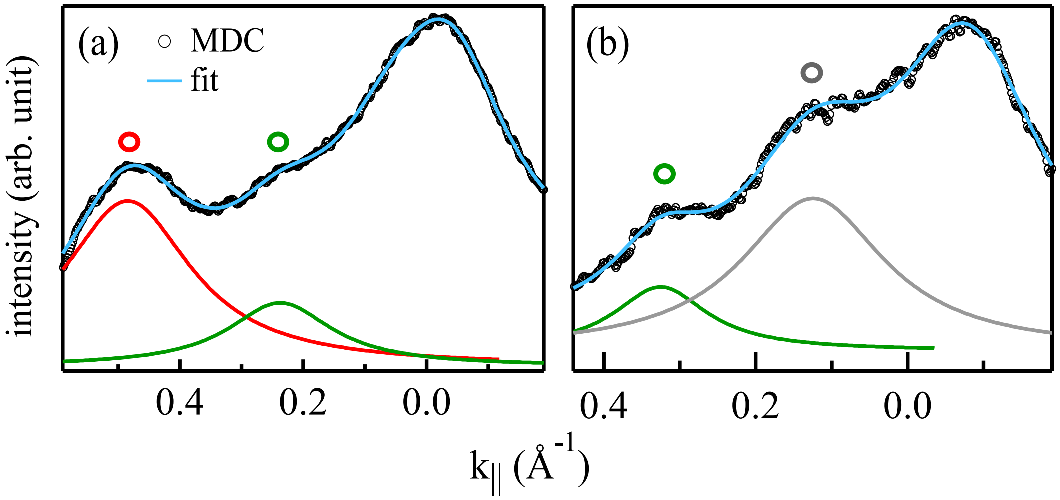


Fig. S 21. Curve fitting of the MDCs obtained from the raw ARPES intensity plot in Fig. 5(a) of the main manuscript shown for example at $E$= (a) 0.25 eV and (b) 0.55 eV. The MDCs are fitted with Lorentzian functions, the fitted curve is shown in cyan color. In panel **a** red (green) open circle and the maximum of the curve represents the peak position of outer (inner) hole band. In panel **b**, green (gray) open circle and the maximum of the curve represents the peak position of the inner hole (inverted parabolic) band.

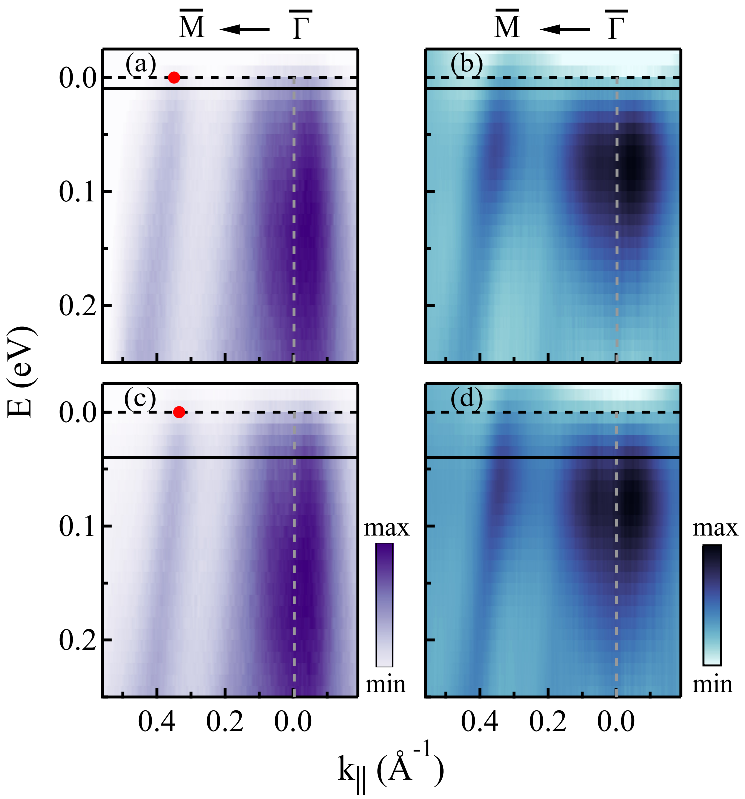


Fig. S 22. ARPES intensity plot and its second derivative plot after (a, b) 10 sec and (c, d) 30 sec potassium deposition on stanene, respectively. Red circles in panels **a** and **c** indicate the position of the outer hole band at $E_F$ obtained from fitting the MDC. The black solid line is the $E_F$ position before K deposition.

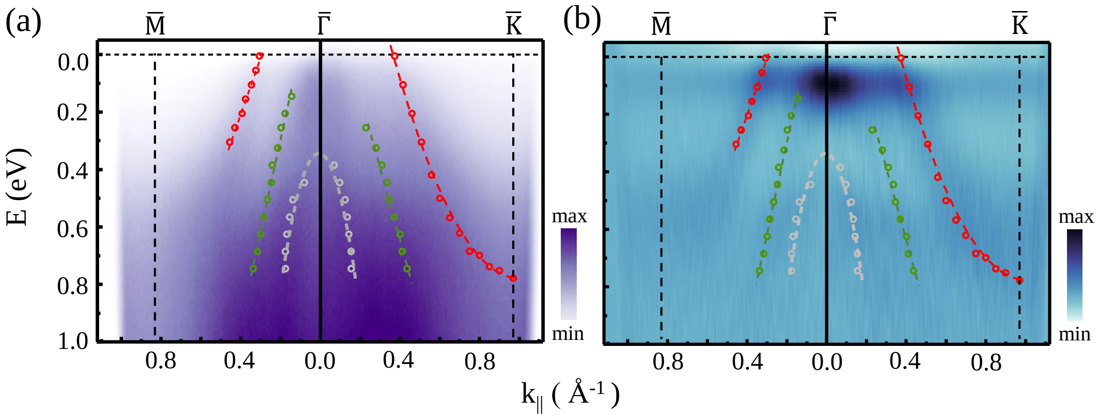


Fig. S 23. (a) Raw and (b) second derivative intensity plots towards the $\overline{M}$-$\overline{\Gamma}$-$\overline{K}$ direction up to $\overline{M}$ and $\overline{K}$ points. This intensity plot was measured at room temperature and has slightly inferior statistics in comparison to the data in Fig. The bands obtained from Fig. 5 are superimposed.

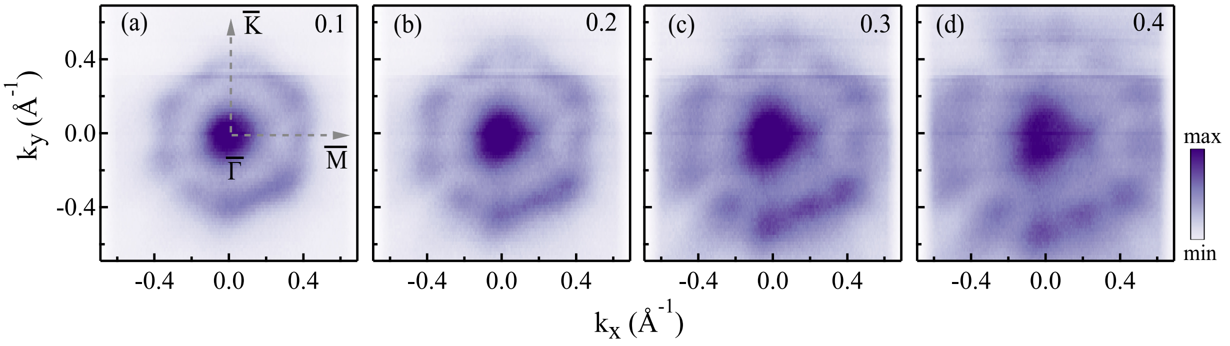


Fig. S 24. (a-d) $k_x$-$k_y$ isosurface plots for $E$ varying from 0.1 to 0.4 eV, as shown in the upper right corner of each panel. The segmentation in the isosurface plot with lower intensity in between $\overline{K}$ and $\overline{M}$ points could be related to characteristic dispersion of the outer band. These plots are obtained by averaging over ±15 meV for each $E$.

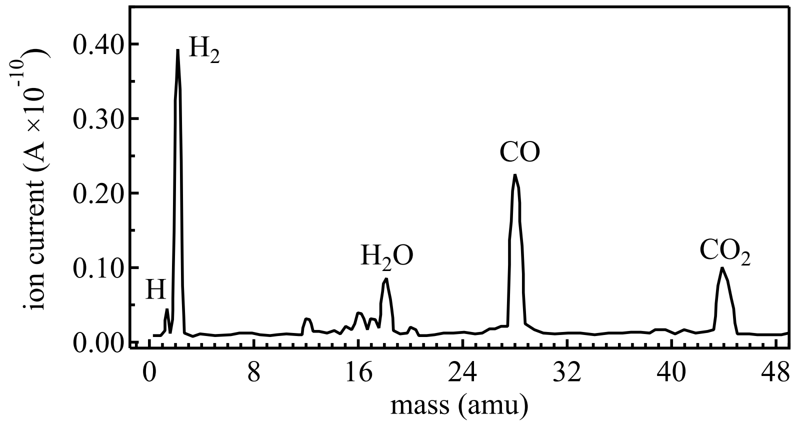


Fig. S 25. A residual mass spectrum recorded with a quadrupole mass spectrometer mounted on the preparation chamber where stanene was grown. The origin of the various dominant peaks is indicated, demonstrating that hydrogen is the most prevalent residual gas.

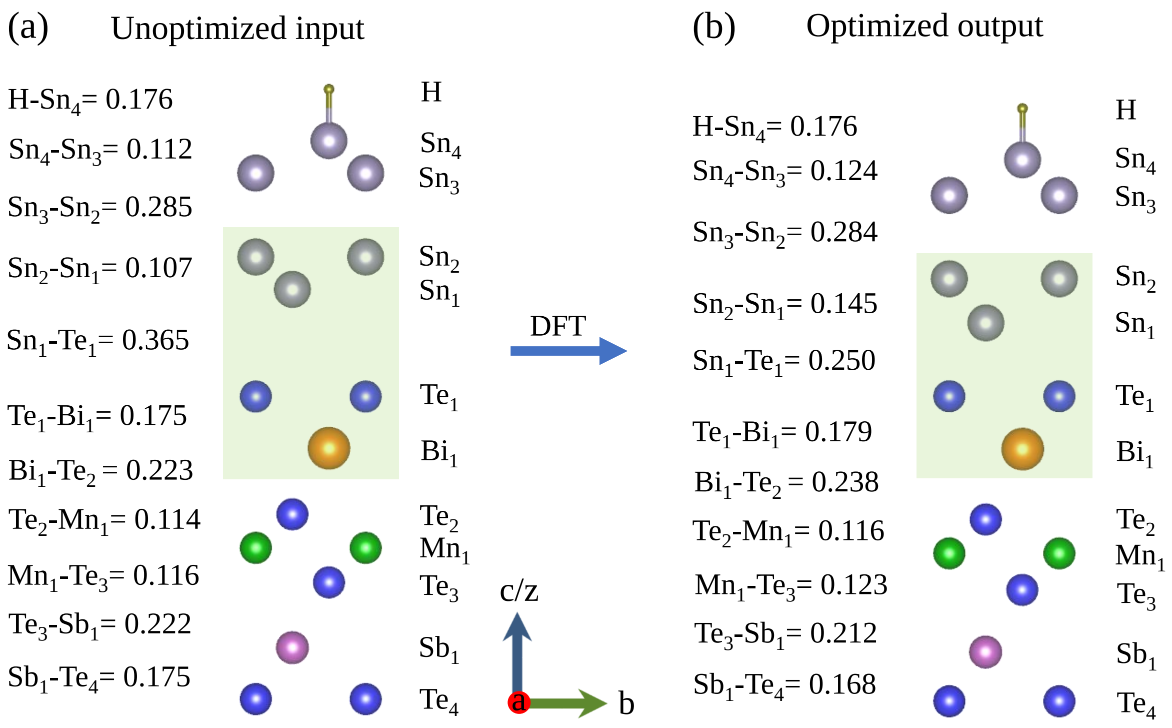


Fig. S 26. (a) The unoptimized input structure and (b) the optimized output structure of **"S+BL+H"** DFT calculation for monolayer stanene on MBST including BL (green shading) and H passivation (topmost layer). The labeled atoms are represented by size-scaled circles of various colors, as in Fig. 5(h) of the main manuscript. Both the structures have been drawn in the same scale using the VESTA program [2]. The separations between the adjacent layers are indicated for both the structures in nm.

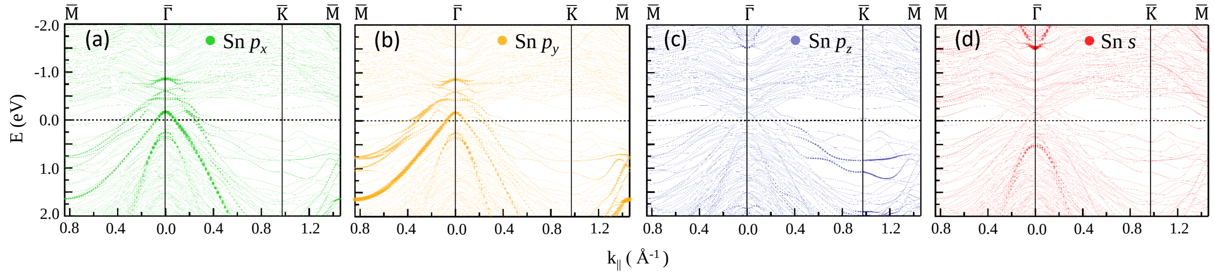


Fig. S 27. The Sn (a) $p_x$, (b) $p_y$, (c) $p_z$, and (d) $s$ orbital character of the bands for the **"S+BL+H"** DFT calculation for monolayer stanene on MBST including BL and H passivation.

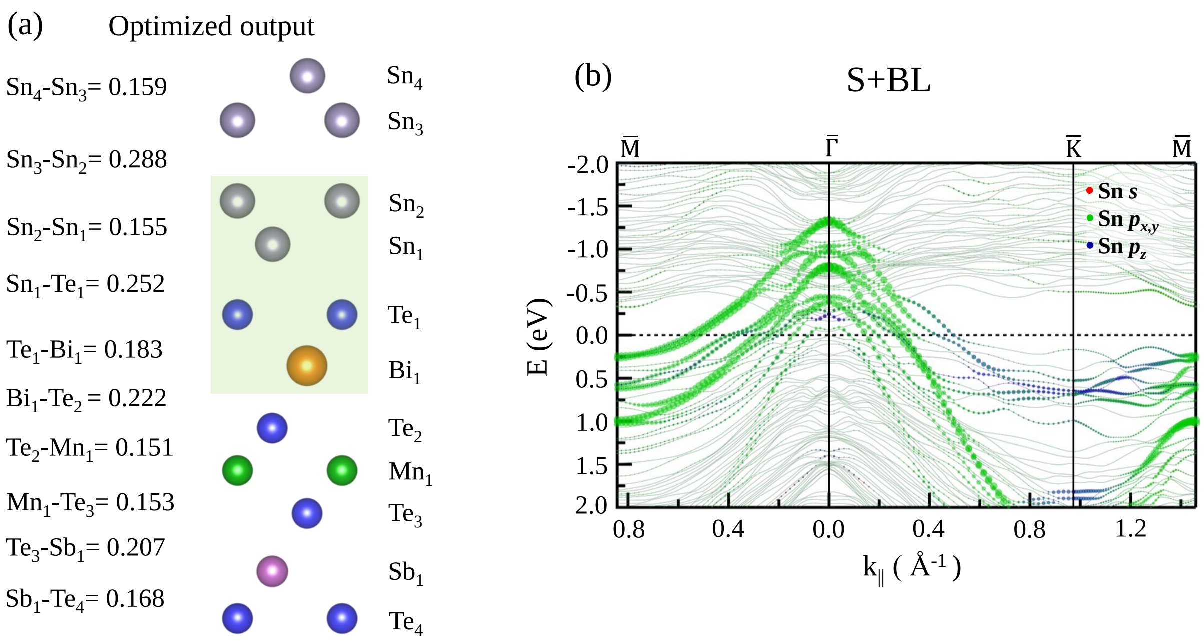


Fig. S 28. (a) The optimized output structure of **"S+BL"** DFT calculation for monolayer stanene on MBST including a BL (green shading) but without H passivation. The labeled atoms are represented by size-scaled circles of various colors, as in Fig. 5(h) of the main manuscript. The separations between the adjacent layers are indicated in nm. (b) The calculated band dispersion including SOC for **"S+BL"** along $\overline{M}$-$\overline{\Gamma}$-$\overline{K}$-$\overline{M}$ directions. The bands of Sn $p_{x,y}$, $p_z$, and $s$ character are highlighted.

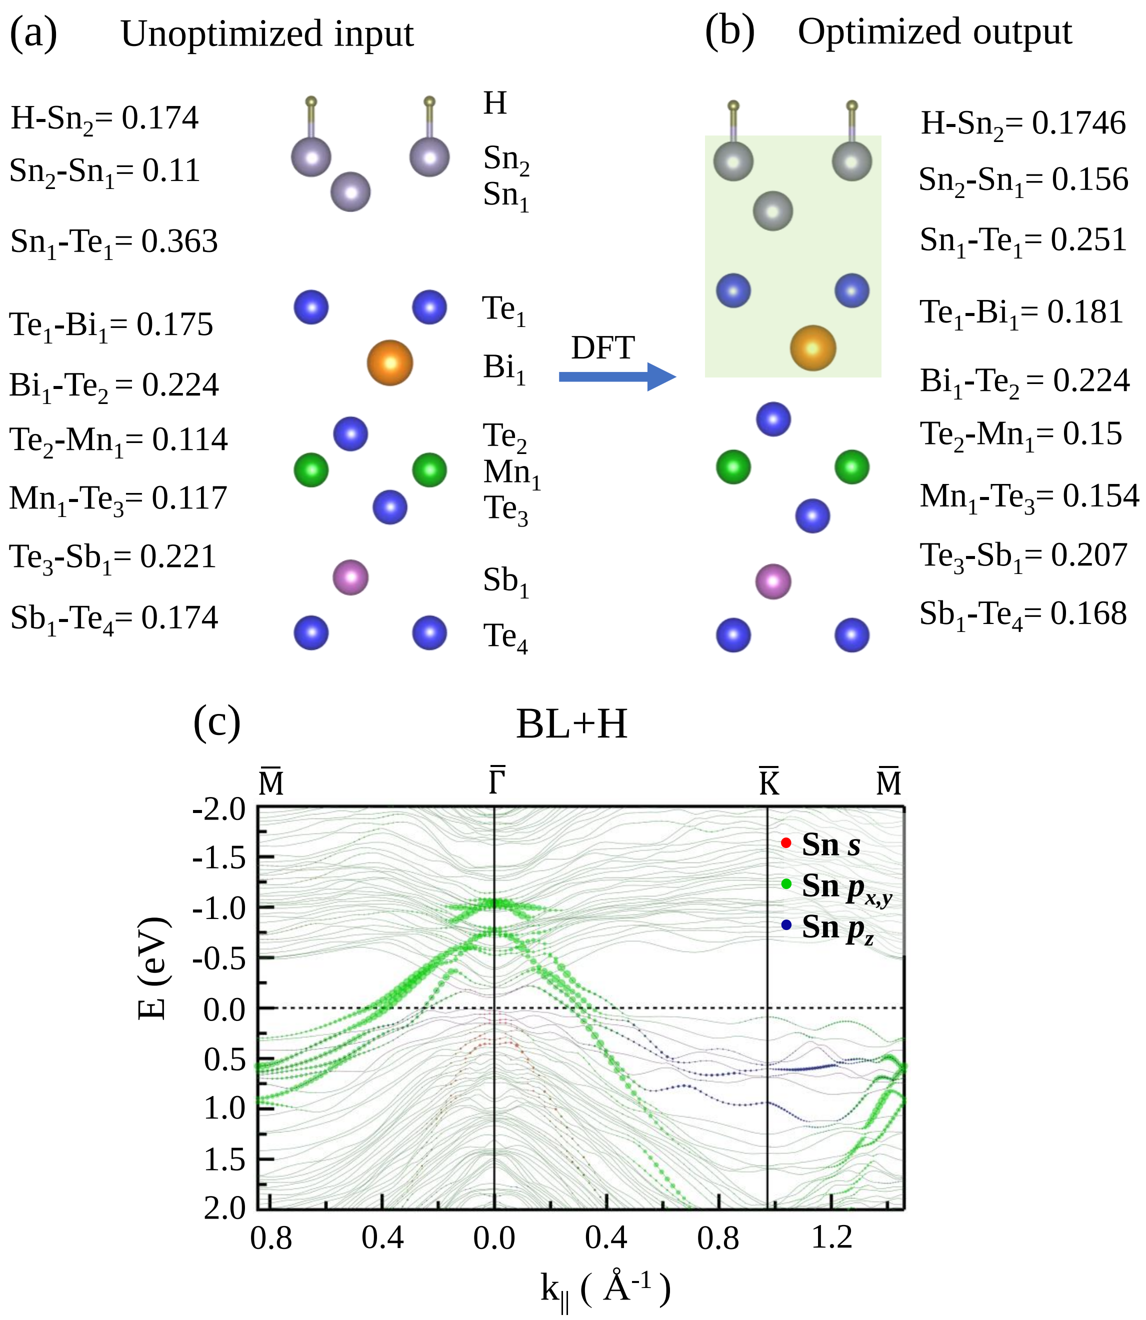


Fig. S 29. (a) The unoptimized input structure and (b) the optimized output structure of **"BL+H"** DFT calculation for BL (green shading) on MBST including H passivation (topmost layer). Both the structures have been drawn in the same scale using the VESTA program [2]. The labeled atoms are represented by size-scaled circles of various colors, as in Fig. 5(h) of the main manuscript. The separations (in nm) between the adjacent layers are indicated for both panels, **a** and **b**. (c) The calculated band dispersion including SOC for **"BL+H"** along $\overline{M}$-$\overline{\Gamma}$-$\overline{K}$-$\overline{M}$ directions. The bands of Sn $p_{x,y}$, $p_z$, and $s$ character are highlighted.

[1] J.-Q. Yan, S. Okamoto, M. A. McGuire, A. F. May, R. J. McQueeney, and B. C. Sales, *Evolution of structural, magnetic, and transport properties in* $MnBi_{2-x}Sb_xTe_4$, Phys. Rev. B **100**, 104409 (2019).

[2] K. Momma and F. Izumi, *VESTA 3 for three-dimensional visualization of crystal, volumetric and morphology data,* J. Appl. Crystallogr. **44**, 1272 (2011).
